# Supplementary material for: Theoretically Efficient Parallel Graph Algorithms Can Be Fast and Scalable
Source: arXiv:1805.05208 source file (2019-08-21)
Supplement: Supplementary file 1 [file additional-techniques.tex]

\section{Additional Techniques}\label{sec:additionaltechniques}
